# Supplementary material for: GMKF: Generalized Moment Kalman Filter for Polynomial Systems with Arbitrary Noise
Source: arXiv:2403.04712 source file (2024-03-08)
Supplement: Supplementary file 1 [file Appendix.tex]

% \clearpage

\begin{appendices}

\section{Auxiliary Matrices }
\label{apx:aux_mat}
We now introduce two sets of symmetric matrices $\left\{\M{B}\right\}$ and $\left\{\M{B}^{\perp}\right\}$. 
We first introduce the auxiliary matrix $\M B_{\gamma}$ to form the moment matrix given the monomial $\M{x}^{\gamma}$:
\begin{equation}
    \M{B}_{\gamma} := \frac{1}{C_{\gamma}} \sum_{\gamma = \alpha + \beta} \ve_{\alpha} \ve^{\transpose}_{\beta},\ \  C_{\gamma}:= { \left| \left\{ (\alpha, \beta) | \gamma = \alpha + \beta \right\}  \right|  },
\end{equation}
where $\ve_\alpha \in \mathbb{R}^{s(r, n) \times 1}$ is the canonical basis corresponding to the $n$-tuples $\alpha \in \mathbb{N}_r^n$ and $C_{\gamma}$ is the normalizing factor. Thus, the moment matrix can be formulated by:
\begin{equation}
    \M{M}_r(\M x) = \sum_{\gamma} C_\gamma \M{B}_{\gamma} \M x^{\gamma}, \gamma \in \mathbb{N}^n_{2r}.
\end{equation}
% Conversely, we can extract the term of $\M{M}_r(y)$ via
% \begin{equation}
% x^{\gamma} = \langle B_\gamma, \M{M}_r(\M x) \rangle.
% \end{equation}
% We then define the orthogonal complement of $\left\{B\right\}$ considering the inner product as the trace function:
% To construct $\{\M{B}^{\perp}\}$, 
We first define the symmetric matrix:
\begin{equation}
    \M{E}_{\alpha, \beta} = \ve_{\alpha}\ve_{\beta}^{\transpose} + \ve_{\beta}\ve_{\alpha}^{\transpose},
\end{equation}
Then we construct $\{\M{B}^{\perp}\}$ to enforce the moment matrix constraints:% given an semidefinite matrix $X \succeq 0$: 
\begin{equation}
   % \left\{ B^{\perp}_{\alpha, \beta} | \langle B^{\perp}_{\alpha, \beta}, B_{\alpha} \rangle, \forall \gamma \in \mathbb{N}^n_{2r} , \alpha + \beta = \gamma \right\}.
   \begin{aligned}
       &\M{B}^{\perp}_{\gamma, \alpha} = \M{E}_{\bar{\alpha}, \bar{\beta}} - \M{E}_{{\alpha}, {\beta}}, \\ 
       % &B^{\perp}_{\gamma, \alpha} = e_{\bar{\alpha}}e_{\bar{\beta}}^{\transpose} + e_{\bar{\beta}}e_{\bar{\alpha}}^{\transpose}  - e_{\alpha}e_{\beta}^{\transpose} - e_{\beta}e_{\alpha}^{\transpose}, \\ 
       &\alpha + \beta = \gamma, \alpha > \bar{\alpha}, \alpha \ge \beta, % \bar{\alpha} + \bar{\beta} = \gamma, 
   \end{aligned}
\end{equation}
where $\bar{\alpha} < \alpha$ is the tuple with the smallest possible lexical orders among all the $\alpha$. 
% We provide a few examples of these matrices in \Cref{apx:B_mat_example}.
% To assist the proof of our main theory, we introduce the following lemmas:

\section{Examples of moment matrix}
\label{apx:B_mat_example}
For $r = 2, n = 2$, we have the moment matrix:
\begin{equation*}
    {\M M}_{2}(\M x) =\left[\begin{array}{cccccc}
1 & x_1 & x_2 & x_1^2 & x_1x_2 & x_2^2 \\
x_1 & x_1^2 & x_1x_2 & x_1^3 & x^2_1x_2 & x_1x_2^2 \\
x_2 & x_1x_2 & x^2_2 & x_1^2x_2 & x_1x^2_2 & x_2^3 \\
x_1^2 & x^3_1 & x_1^2x_2 & x_1^4 & x^3_1x_2 & x_1^2x_2^2 \\
x_1x_2 & x_1^2x_2 & x_1x^2_2 & x_1^3x_2 & x_1^2x_2^2 & x_1x_2^3 \\
x_2^2 & x_1x_2^2 & x^3_2 & x_1^2x_2^2 & x_1x^3_2 & x_2^4 \\
\end{array}\right] .
\end{equation*} 
For $\gamma = (0, 2)$ that corresponds to $x_1^2$, we have:
\begin{equation}
    \M B_{\gamma} = \frac{1}{C_{\gamma}} \begin{bmatrix}
        0 & 0 & 0 & 1 & 0 & 0 \\
        0 & 1 & 0 & 0 & 0 & 0 \\
        0 & 0 & 0 & 0 & 0 & 0 \\
        1 & 0 & 0 & 0 & 0 & 0 \\
        0 & 0 & 0 & 0 & 0 & 0 \\
        0 & 0 & 0 & 0 & 0 & 0 \\
    \end{bmatrix}, C_{\gamma} = \frac{1}{3},
\end{equation}
% \begin{equation}
%     B_{\gamma} = \frac{1}{C_{\gamma}} \begin{bmatrix}
%         0 & 0 & 0 & 0 & 1 & 0 \\
%         0 & 0 & 1 & 0 & 0 & 0 \\
%         0 & 1 & 0 & 0 & 0 & 0 \\
%         0 & 0 & 0 & 0 & 0 & 0 \\
%         1 & 0 & 0 & 0 & 0 & 0 \\
%         0 & 0 & 0 & 0 & 0 & 0 \\
%     \end{bmatrix}
% \end{equation}
and
\begin{equation}
\begin{aligned}
    \M B^{\perp}_{\gamma, \alpha} &= \M e_{\bar{\alpha}}\M e_{\bar{\beta}}^{\transpose} + \M e_{\bar{\beta}}\M e_{\bar{\alpha}}^{\transpose}  - (\M e_{\alpha}\M e_{\beta}^{\transpose} + \M e_{\beta}\M e_{\alpha}^{\transpose}) \\
    &= \M E_{\bar{\alpha}, \bar{\beta}} - \M E_{{\alpha}, {\beta}} \\
    &= \begin{bmatrix}
        0 & 0 & 0 & -1 & 0 & 0 \\
        0 & 2 & 0 & 0 & 0 & 0 \\
        0 & 0 & 0 & 0 & 0 & 0 \\
        -1 & 0 & 0 & 0 & 0 & 0 \\
        0 & 0 & 0 & 0 & 0 & 0 \\
        0 & 0 & 0 & 0 & 0 & 0 \\
    \end{bmatrix},
\end{aligned}
\end{equation}
where the canonical basis is chosen as: 
\begin{equation}
\begin{aligned}
     \M e_{\bar{\alpha}} &= \begin{bmatrix}
        0 & 1 & 0 & 0 & 0 & 0
    \end{bmatrix}, \M e_{\bar{\beta}} &= \begin{bmatrix}
        0 & 1 & 0 & 0 & 0 & 0
    \end{bmatrix},\\
    \M e_{{\alpha}} &= \begin{bmatrix}
        0 & 0 & 0 & 1 & 0 & 0
    \end{bmatrix}, \M e_{{\beta}} &= \begin{bmatrix}
        1 & 0 & 0 & 0 & 0 & 0
    \end{bmatrix}. \\
\end{aligned}
\end{equation}
Via enforcing the constraints:
\begin{equation}
    \langle \M B^{\perp}_{\gamma, \alpha}, \M X \rangle = 0, \M X \succeq 0,
\end{equation}
we can guarantee that all the entries corresponding to $x_1^2$ are identical. 
% \begin{equation}
% \begin{aligned}
%     B_{\gamma, \alpha_1} &= \begin{bmatrix}
%         0 & 0 & 0 & -1 & 0 & 0 \\
%         0 & 1 & 0 & 0 & 0 & 0 \\
%         0 & 0 & 0 & 0 & 0 & 0 \\
%         0 & 0 & 0 & 0 & 0 & 0 \\
%         0 & 0 & 0 & 0 & 0 & 0 \\
%         0 & 0 & 0 & 0 & 0 & 0 \\
%     \end{bmatrix} \\ 
%     B_{\gamma, \alpha_2} &= \begin{bmatrix}
%         0 & 0 & 0 & 0 & 0 & 0 \\
%         0 & 1 & 0 & 0 & 0 & 0 \\
%         0 & 0 & 0 & 0 & 0 & 0 \\
%         -1 & 0 & 0 & 0 & 0 & 0 \\
%         0 & 0 & 0 & 0 & 0 & 0 \\
%         0 & 0 & 0 & 0 & 0 & 0 \\
%     \end{bmatrix}
% \end{aligned}
% \end{equation}
\section{\Cref{lemma:B_orthogonal}}
\label{apx:proof:B_orthogonal}
\begin{restatable}{lemmma}{lemmaBorthogonal}
\label{lemma:B_orthogonal}
    All $\{\M B^{\perp}\}$ and $\{\M B\}$ form a basis for matrix $\mathbb{R}^{s(r, n) \times s(r, n)}$ and they are orthogonal complement.
\end{restatable}
\begin{proof}

To show the orthogonality, for $\gamma \neq \gamma'$, $$\left\langle \M B_{\gamma, \alpha}^{\perp}, \M B_{\gamma'} \right\rangle = 0, \forall \alpha,$$ is obvious as non-zero entry will not appear in the identical locations. 
For $\gamma = \gamma'$, we have:
\begin{equation}
\label{eq:B_orthogonal}
\begin{aligned}
    \left\langle \M B_{\gamma, \alpha}^{\perp}, \M B_{\gamma} \right\rangle &= \langle \M E_{\bar{\alpha}, \bar{\beta}} - \M E_{{\alpha}, {\beta}},  \frac{1}{C_{\gamma}} \sum_{\gamma = \alpha' + \beta'} \M e_{\alpha'} \M e^{\transpose}_{\beta'} \rangle \\
    &= \langle \M e_{\bar{\alpha}}\M e_{\bar{\beta}}^{\transpose} + \M e_{\bar{\beta}}\M e_{\bar{\alpha}}^{\transpose},  \frac{1}{C_{\gamma}} \sum_{\gamma = \alpha' + \beta'} \M e_{\alpha'} \M e^{\transpose}_{\beta'}\rangle \\ & \quad -  \langle \M e_{{\alpha}}\M e_{{\beta}}^{\transpose} + \M e_{{\beta}}\M e_{{\alpha}}^{\transpose},  \frac{1}{C_{\gamma}} \sum_{\gamma = \alpha' + \beta'} \M e_{\alpha'} \M e^{\transpose}_{\beta'} \rangle \\
    & = \frac{2}{C_{\gamma}} - \frac{2}{C_{\gamma}} = 0.
\end{aligned}.
% \begin{aligned}
%     \left\langle B^{\perp}_{\gamma, \alpha}, M_r(x) \right\rangle &= \langle B^{\perp}_{\gamma, \alpha}, \sum_{\gamma} C_\gamma B_{\gamma} x^{\gamma}\rangle = 0  \\
%       & \Rightarrow \left\langle B^{\perp}_{\gamma, \alpha}, B_{\gamma} \right\rangle = 0 \\
% \end{aligned}
\end{equation} % , \gamma
% \tsl{Add a remark that $B$ and $B^{\perp}$ are sufficient to generate any matrix.} \tsl{$B$ and $B^{\perp}$ are orthogonal to each other and can generate any matrix, thus is an element-wise basis.}

To show $\left\{\M B\right\} \cup \left\{\M B^{\perp}\right\}$ form a basis for symmetric matrix $\mathbb{R}^{s(r, n) \times s(r, n)}$, by the structure of $\{\M{B}\}$ we have:
\begin{equation}
\label{eq:B_basis}
    \M e_{\bar{\alpha}}\M e^{\transpose}_{\bar{\beta}} = C_{\gamma}\M B_{\gamma} - \sum_{\gamma = \alpha + \beta}\M e_{\alpha}\M e_{\beta}^{\transpose}.
\end{equation}
Then, we have
\begin{equation}
\begin{aligned}
    \M E_{\bar{\alpha}, \bar{\beta}} &= 2C_{\gamma}\M B_{\gamma} - \sum_{\gamma = \alpha + \beta, \alpha \ge \beta}\M E_{\alpha, \beta} \\
    &= 2C_{\gamma}\M B_{\gamma} - \sum_{\gamma = \alpha + \beta, \alpha \ge \beta}(\M B^{\perp}_{\gamma, \alpha} - \M E_{\bar{\alpha}, \bar{\beta}}).
\end{aligned}
\end{equation}
Finally, we show that 
\begin{equation}
\label{eq:E_alpha_beta}
    \M E_{\bar{\alpha}, \bar{\beta}} = \frac{2C_{\gamma}}{C_{\gamma}^{'} + 1}\M{B}_{\gamma} - \frac{1}{C_{\gamma}^{'} + 1}\sum_{\gamma = \alpha + \beta, \alpha \ge \beta}\M{B}_{\gamma, \alpha}^{\perp}
\end{equation}
with $C_{\gamma}^{'} = |\{ (\alpha, \beta) | \alpha + \beta = \gamma, \alpha \ge \beta \} |$.

By the definition of $\{\M{B}^{\perp}\}$, $\forall \alpha, \beta$ and $\alpha + \beta = \gamma$, we have:
\begin{equation}
\begin{aligned}
    \M E_{\alpha, \beta} &= \M E_{\bar{\alpha}, \bar{\beta}} - \M B^{\perp}_{\gamma, \alpha}
    % &=\frac{C_{\gamma}}{(C_{\gamma} + 1)} B_{\gamma} + \frac{1}{(C_{\gamma} + 1)}\sum_{\gamma = \alpha' + \beta'}B^{\perp}_{\gamma, \alpha'} - B_{\gamma, \alpha}^{\perp}
\end{aligned}.
\end{equation}
By substituting \eqref{eq:E_alpha_beta}, we show that any entry of the symmetric matrix, i.e. $\M{E}_{\alpha, \beta}$, can be represented by the linear combination of elements in $\left\{\M B\right\} \cup \left\{\M B^{\perp}\right\}$. % \tsl{Need to check the constant.}
\end{proof}

\section{Proof of \Cref{lemma:exist_sos_xi}}
\label{apx:proof:exist_sos_xi}
% \lemmaexistsosxi*
{
\begin{restatable}[Equivalent SOS Polynomial Descriptions]{lemmma}{lemmaexistsosxi}
% \begin{lemma}[Equivalent polynomial]
    \label{lemma:exist_sos_xi}
    Let $\M{Y}_1, \M{Y}_2 \succeq 0$ be two matrices such that $\vv^{\transpose}_r(\M x) \M{Y}_1 \vv^{\transpose}_r(\M x)=\vv^{\transpose}_r(\M x) \M{Y}_2 \vv^{\transpose}_r(\M x), \forall \M x$, i.e., the polynomials corresponding to $\M{Y}_1$ and $\M{Y}_2$ are identical. Then, there exists a matrix $\M{\xi}$ such that $\M{Y}_1=\M{Y}_2+{\M{\xi}}$,
    where $\M{\xi}=\sum_{i} \mu_{i} \M{B}^{\perp}_{i}, \mu_i \in \mathbb{R}$. % \tsl{This lemma does not require $\M Y\ge 0$.}
    % and $\xi = \sum_{(\gamma, \alpha)}\mu_{\gamma, \alpha}B_{\gamma, \alpha}^{\perp}$. % with $\left\langle{\M{\xi}}, {\M{B}}_{{\gamma}}\right\rangle=0$ for all ${\gamma}$ such
% \end{lemma}
\end{restatable}
}
We provide the proof of \Cref{lemma:exist_sos_xi} based on the fact shown in \Cref{lemma:B_orthogonal} that the $\{\M B\}$ and $\{\M B^{\perp}\}$ are orthogonal complements for positive semidefinite matrix:
\begin{proof}
        \begin{align}
        &\M v^{\transpose}_r(\M x) (\M Y_1-\M Y_2) \M v_r( \M x)=0, \quad \forall \M x \Leftrightarrow  \\
        &\left\langle \M Y_1-\M Y_2, \M v_r( \M x)\M v^{\transpose}_r(\M x)\right\rangle=0, \quad \forall \M x \Leftrightarrow \\
        &\langle \M Y_1-\M Y_2, \sum \M x^{\gamma}\M B_{\gamma}\rangle=0, \quad \forall \M x \Rightarrow \\
        &\left\langle \M Y_1-\M Y_2, {\M B}_{{\gamma}}\right\rangle= 0, \quad \forall \gamma
        \end{align}
% This last implication holds in the reverse direction: if a polynomial $p(\mathbf{z})$ has all zero coefficients, then it must be the zero polynomial.
As $\left\{\M B^{\perp}\right\}$ and $\left\{\M B\right\}$ are orthogonal complements, $\M\xi$ exists and can be constructed by $\M B^{\perp}$ as
    \begin{equation}
    \label{eq:exist_of_xi}
        \M \xi := \M Y_1 - \M Y_2 = \sum_{i} \mu_{i} \M B^{\perp}_{i}
    \end{equation}
\end{proof}
This proof is equivalent to the version in \cite{cosse2021stable} but with the application of $\left\{ \M B^{\perp} \right\}$.

\section{Example of Extended Polynomial System and Its Affine Form}
\label{appx:momcond_linear}
We provide an example of the extended polynomial system and transform it to the affine form \eqref{eq:gmm_cond} used in \eqref{eq:BPUE}:

Consider a linear observation $\M x, \M y \in \mathbb{R}^2$ function:
\begin{equation}
\begin{aligned}
    y_1 - x_1 &= w_1 \\
    y_2 - x_2 &= w_2
\end{aligned}
\end{equation}
We consider the extended system with $r=2$ and the higher-order terms of $\M y, \M x, \M w$ are:
\begin{equation}
    \begin{aligned}
        \M \phi_r(\M y) = \begin{bmatrix}
            y_1\\y_2\\y_1y_2\\y_1^2\\y_2^2
        \end{bmatrix},
        \M \phi_r(\M x) = \begin{bmatrix}
            x_1\\x_2\\x_1x_2\\x_1^2\\x_2^2
        \end{bmatrix},
        \M \phi_r(\M v) = \begin{bmatrix}
            w_1\\w_2\\w_1w_2\\w_1^2\\w_2^2
        \end{bmatrix}
    \end{aligned}.
\end{equation}
We further have:
\begin{equation}
\begin{aligned}
     \M \phi_r(\M y - \M x) &= \begin{bmatrix}
            y_1 - x_1\\
            y_2 - x_2\\
            (y_1-x_1)(y_2-x_2)\\
            (y_1-x_1)^2\\
            (y_2-x_2)^2
        \end{bmatrix}\\ &= \begin{bmatrix}
            y_1 - x_1\\
            y_2 - x_2\\
            y_1y_2 + x_1x_2 - y_1x_2 - y_2x_1\\
            y_1^2  + x_1^2 - 2y_1x_1\\
            y_2^2  + x_2^2 - 2y_2x_2
        \end{bmatrix}
\end{aligned}
\end{equation}
We then use an affine function to express the moment condition:
\begin{equation}
    \boldsymbol m(\M y, \M x) := \vb(\M y) - \M{A}(\M y)\M \phi_r(\M x) = \vv, \M V = \operatorname{Cov}[\vv],
\end{equation}
where
\begin{equation}
\begin{aligned}
    \M b(\M y) &= \begin{bmatrix}
        y_1 - \mathbb{E}[w_1]\\
        y_2 - \mathbb{E}[w_2]\\
         y_1y_2 - \mathbb{E}[w_1w_2]\\
        y_1^2 - \mathbb{E}[w_1^2]\\
        y^2_2 - \mathbb{E}[w_2^2]\\
    \end{bmatrix},     \M v = \begin{bmatrix}
        w_1 - \mathbb{E}[w_1]\\
        w_2 - \mathbb{E}[w_2]\\
         w_1w_2 - \mathbb{E}[w_1w_2]\\
        w_1^2 - \mathbb{E}[w_1^2]\\
        v^2_2 - \mathbb{E}[w_2^2]\\
    \end{bmatrix}, \\
    \M A(\M y) &= \begin{bmatrix}
        1&0&0&0&0\\
        0&1&0&0&0\\
        y_2&y_1&-1&0&0\\
        2y_1&0&0&-1&0\\
        0&2y_2&0&0&-1
    \end{bmatrix}.
\end{aligned}
\end{equation}

\section{Proof of \Cref{prop:blue-quad}}
\propbluequad*
\begin{proof}

    In \BLUE, we assume that $\M{A}$ has full column rank \cite{humpherys2012fresh}. Then we expand the cost of \BLUE as:
    \begin{equation}
    \begin{aligned}
        ||\M A \M x - \M b||_{\M{V}^{-1}}^2 &= \M x^\transpose \M A^\transpose \M{V}^{-1} \M A \M x - 2\M x^\transpose \M A^\transpose\M{V}^{-1}\M b + \M b ^\transpose \M{V}^{-1}\M b.
    \end{aligned}
    \end{equation}

    By the first-order optimality condition, the minimum is achieved when $\hat{\M x} = (\M A^\transpose \M{V}^{-1} \M A)^{-1}\M A^\transpose \M{V}^{-1} \M b$. Thus, we can write the quadratic belief as follows and verify that it is identical to the original cost function (up to a constant):
    \begin{equation}
        \begin{aligned}
            &\quad||\M x - (\M A^\transpose \M{V}^{-1} \M A)^{-1}\M A^\transpose \M{V}^{-1} \M b||^2_{\M A^\transpose \M{V}^{-1} \M A}\\
            &= \left(\M x - (\M A^\transpose \M{V}^{-1} \M A)^{-1}\M A^\transpose \M{V}^{-1} \M b\right)^\transpose\M A^\transpose \M{V}^{-1} \M A\\
            &\quad\cdot\left(\M x - (\M A^\transpose \M{V}^{-1} \M A)^{-1}A^\transpose \M{V}^{-1} \M b\right)\\
            &=(\M x^\transpose(\M A^\transpose \M{V}^{-1} \M A) - \M b^\transpose \M{V}^{-1} \M A) \\
            &\quad \cdot (\M x - (\M A^\transpose \M{V}^{-1} \M A)^{-1}\M A^\transpose \M{V}^{-1} \M b)\\
            &= \M x^\transpose\M A^\transpose \M{V}^{-1} \M A\M x - 2\M x^\transpose \M A^\transpose\M{V}^{-1}\M b\\
            &\quad+ \M b^\transpose\M{V}^{-1} \M A(\M A^\transpose \M{V}^{-1} \M A)^{-1}\M A^\transpose \M{V}^{-1} \M b.
        \end{aligned}
    \end{equation}

Thus, we can express \BLUE as the sum of quadratic belief and a constant term:
\begin{equation}
    \begin{aligned}
         \| \M{A}\M{x} - \M{b} \|^2_{\M{V}^{-1}} &= \| \M x - \hat{\M x} \|^2_{\M{\Sigma}^{-1}} + \hat{\rho},
         \end{aligned}
\end{equation}
where 
\begin{equation}
    \begin{aligned}
         \M{\Sigma} &:= (\M A^\transpose \M{V}^{-1} \M A)^{-1},\\
         \hat{\M x} &:= ( \M A^\transpose \M{V}^{-1} \M A)^{-1} \M A^\transpose \M{V}^{-1} \M b,\\
         \hat{\rho} &:= \M b^\transpose \M{V}^{-1} \M b - \M b^\transpose\M{V}^{-1}\M A(\M A^\transpose \M{V}^{-1} \M A)^{-1}\M A^\transpose \M{V}^{-1} \M b.
    \end{aligned}
\end{equation}
\end{proof}

\section{Proof of \Cref{theorem:SDP=POP}}
\label{apx:SDP=SOS}
\theoremSDPPOP*
% 0Now we show that, under the rank-1 assumption, the SoS form induced from the optimality condition can be used to construct the prior factor in the moment matching problem. 

% Now, it suffices to show the equivalence of the SDP primal solution and the duality certificate.
% \tsl{Need to show why it is sufficient to construct $\xi$ by $B^{\perp}$ .} \tsl{Need some basis theorem maybe.}
% \begin{theorem}[Dual certificate as the prior factor]
%     % The \ref{SDP} has rank-1 optimal solutions if and only if the SOS global optimality condition is satisfied and $\sigma_0(x)$ is an prior factor of the moment matching problem.
%     % Suppose that the solution
%     % The dual SOS $\sigma_0(x)$ is in the form of prior factor if and only if the first-order optimality condition is satisfied. 
%     Suppose the unique optimal solution of \ref{prob:pop} is $\bar{x}$. The \ref{prob:pop_sdp} corresponding to \ref{prob:pop} has rank-1 optimal solution $v_r(\bar{x})v_r(\bar{x})^{\transpose}$. Then the dual certificate is of the form \mbox{$\sigma_0(x) = \| v_r(\M x) - v_r(\bar{x}) \|_{W}^2$}, $W>0$, iff the first order optimality condition \ref{def:kkt_sdp} is satisfied. 
% \end{theorem}
\begin{proof}

    Before the main proof, We first convert the optimality condition in \Cref{def:kkt_sdp} to its polynomial form.  Taking inner products on both sides of the stationary condition 1) in \Cref{def:kkt_sdp} with ${\M X}:= \M v_r(\M x)\M v^{\transpose}_r(\M x)$:
    $$\langle\M Y, \M{X} \rangle= \langle \M C + \sum_{j} \lambda_{j} \M G_{j} + \left( \sum_{i}\mu_{i} \M B^{\perp}_{i} - \rho \M e_1\M e_1^{\transpose} \right), \M{X} \rangle$$
    we have the optimality condition in the polynomial form \cite{lasserre2001global, lasserre2015introduction}:
\begin{equation}
    \M v^{\transpose}_r(\M x)\M Y\M v_r(\M x) = p(\M x) + \sum_j h_j(\M x)g_j(\M x) - \rho,
\end{equation}
where the term corresponding to $\M B^{\perp}$ vanishes by its construction, and $h_i(x)$ are the polynomials defined by the localizing matrix $\M G_i$ and its associated multiplier $\lambda_i$. Now we start the main proof. 

    $\Longrightarrow:\;$
    Suppose the dual SOS has the form:
    \begin{equation}
        \begin{aligned}
        \M v^{\transpose}_r(\M x)\hat{\M{Y}}\M v_r(\M x) &= \|\M \phi_r(\M x) - \M \phi_r(\hat{\M x})\|^2_{\M{\Sigma}^{-1}},  \M{\Sigma} \succ 0 
                    % &= p(\M x) + \sum_{k=1}^m h_i(\M x)g_i(\M x) - \rho, \M{\Sigma}^{-1} > 0 
        \end{aligned}.
    \end{equation}
    % {\color{red} are we assuming the shape of Y here? also: is the product below giving zero?}\tsl{Yes, the shape needs to be compatible with $\phi(x)$. The next equation tells how to obtain the SOS belief from a matrix.}
    We have: % Can be expanded as a $s(r, n)\times s(r, n)$ to serve as the dual certificate. 
    % \begin{equation}
    %     \begin{aligned}
    %         & \M v^{\transpose}_r(\M x)\hat{\M{Y}}\M v_r(\M x) \\
    %         &=\begin{bmatrix}
    %         1 \\
    %         \M \phi_r(\M x)
    %     \end{bmatrix}^{\transpose}
    %     \begin{bmatrix}
    %          \M \phi_r(\hat{\M x})^{\transpose}\M{\Sigma}^{-1} \M \phi_r(\hat{\M x}) & -(\M{\Sigma}^{-1}\M \phi_r(\hat{\M x}))^{\transpose} \\
    %         -\M{\Sigma}^{-1}\M \phi_r(\hat{\M x}) & \M{\Sigma}^{-1}
    %     \end{bmatrix}\begin{bmatrix}
    %         1 \\
    %         \M \phi_r(\M x)
    %     \end{bmatrix}
    %     \end{aligned}.
    % \end{equation}
    % The dual solution can be constructed as 
    $$\hat{\M{Y}}:= \begin{bmatrix}
        \M \phi_r(\hat{\M x})^{\transpose}\M{\Sigma}^{-1}\M \phi_r(\hat{\M x}) & -(\M{\Sigma}^{-1}\M \phi_r(\hat{\M x}))^{\transpose} \\
            -\M{\Sigma}^{-1}\M \phi_r(\hat{\M x}) & \M{\Sigma}^{-1}
        \end{bmatrix},$$
    and a candidate primal solution:
    $$
        \hat{\M{X}}:= \begin{bmatrix}
            1 \\
            \M \phi_r(\hat{\M x})
        \end{bmatrix}\begin{bmatrix}
            1 \\
            \M \phi_r(\hat{\M x})
        \end{bmatrix}^{\transpose}.
    $$
    It is straightforward to verify that $Rank(\hat{\M{X}}) = 1$, $Rank(\hat{\M{Y}}) = s(r, n) - 1$, and $\langle \hat{\M{X}}, \hat{\M{Y}} \rangle = 0$. 
    Given the optimality condition in polynomial form, we have
    $$\M v^{\transpose}_r(\M x)\hat{\M{Y}}\M v_r(\M x) = \M v^{\transpose}_r(\M x)\left(\M C -\rho \M e_1\M e_1^{\transpose} + \sum_{j} \lambda_{j} \M G_{j}\right)\M v_r(\M x).$$ By Lemma \ref{lemma:exist_sos_xi}, there must exist $\M \xi = \sum_{i} \mu_{i} \M B^{\perp}_{i}$ that enables the matrix on both sides corresponds to identical polynomials: 
    $$\hat{\M{Y}} = \M C - \rho \M e_1\M e_1^{\transpose} + \sum_{j} \lambda_{j} \M G_{j} + \M \xi.$$
    Now we have shown that the dual solution $\hat{\M{Y}}$ also satisfies the optimality condition in \Cref{def:kkt_sdp}.
    
     $\Longleftarrow:\;$
    If the SDP has a rank-1 solution and satisfies the strict complementary condition in \Cref{def:kkt_sdp}, we have $\langle \hat{\M{X}}, \hat{\M{Y}}\rangle = 0$, with $\operatorname{Rank}(\hat{\M{X}}) = 1, \operatorname{Rank}(\hat{\M{Y}}) = s(r, n) - 1$. By SVD of $\hat{\M{Y}}$, we have:

    \begin{equation}
        \begin{aligned}
            \hat{\M{Y}} &= \sum_{i=1}^{s(r, n) - 1} \delta_i \M f_i\M f_i^{\transpose} \\
              &= \begin{bmatrix}
                  \sqrt{\delta_1}\M f^{\transpose}_1 \\
                  \vdots \\
                  \sqrt{\delta_{s(r, n) - 1}}\M f^{\transpose}_{{s(r, n) - 1}} \\
              \end{bmatrix}^{\transpose}
              \begin{bmatrix}
                  \sqrt{\delta_1}\M f^{\transpose}_1 \\
                  \vdots \\
                  \sqrt{\delta_{s(r, n) - 1}}\M f^{\transpose}_{{s(r, n) - 1}} \\
              \end{bmatrix} \\
              &=: \M F\M F^{\transpose},
        \end{aligned}
    \end{equation}
    with $\M f_i \in \mathbb{R}^{s(r, n)\times 1}$ are mutually orthogonal and $\delta_i > 0$ the non-trivial singular values. Similarly, by SVD of $\hat{\M{X}}$ and $\langle \hat{\M{X}}, \hat{\M{Y}} \rangle = 0$, we have:
    \begin{equation}
        \hat{\M{X}} =  \begin{bmatrix}
            1 \\
            \M \phi_r(\hat{\M x})
        \end{bmatrix}\begin{bmatrix}
            1 \\
            \M \phi_r(\hat{\M x})
        \end{bmatrix}^{\transpose}, \begin{bmatrix}
            1 \\
            \M \phi_r(\hat{\M x})
        \end{bmatrix}^{\transpose}\M f_i = 0, \forall i.
    \end{equation}
Let us partition $\M F$ by:
    \begin{equation}
    \begin{aligned}
        \M F &= \begin{bmatrix}
            \M f \\
            \bar{\M F}
        \end{bmatrix}
    \end{aligned}
    \end{equation}
where $\M f\in\mathbb{R}^{1\times (s(r,n) - 1) }, \bar{\M F} \in \mathbb{R}^{(s(r, n) - 1) \times (s(r, n) - 1) }$. By the strict complementary condition $\langle \hat{\M{X}}, \hat{\M{Y}} \rangle = 0$, we have
    \begin{equation}
    \begin{aligned}
        \M F^{\transpose}\begin{bmatrix}
            1 \\
            \M \phi_r(\hat{\M x})
        \end{bmatrix} &= \begin{bmatrix}
            \M f^{\transpose}, \bar{\M F}^{\transpose}
        \end{bmatrix}\begin{bmatrix}
            1 \\
            \M \phi_r(\hat{\M x})
        \end{bmatrix} \\
        &= \M f^{\transpose} + \bar{\M F}^{\transpose}
            \M \phi_r(\hat{\M x}) = 0.
    \end{aligned}
    \end{equation}
    \begin{equation}
        \M f^{\transpose} = - \bar{\M F}^{\transpose}\M \phi_r(\hat{\M x})
    \end{equation}
    As ${\M f}^{\transpose}$ is a linear combination of the $\bar{\M F}$, $\bar{\M F}$ must have full rank to ensure that $\operatorname{Rank}(\M F) = s(r, n) - 1$. We can then obtain the SOS belief via:
    \begin{equation}
    \begin{aligned}
        &\sigma(\hat{\M{x}}, \M\Sigma)  \\
        &:= \begin{bmatrix}
            1 \\
            \M \phi_r(\M x)
        \end{bmatrix}^{\transpose}\M F\M F^{\transpose}\begin{bmatrix}
            1 \\
            \M \phi_r(\M x)
        \end{bmatrix} \\
        &= \begin{bmatrix}
            1 \\
            \M \phi_r(\M x)
        \end{bmatrix}^{\transpose}
        \begin{bmatrix}
            \M f\M f^{\transpose} & \M f\bar{\M F}^{\transpose} \\
            \bar{\M F}\M f^{\transpose} & {\bar{\M F}\bar{\M F}^{\transpose}}\\
        \end{bmatrix}
        \begin{bmatrix}
            1 \\
            \M \phi_r(\M x)
        \end{bmatrix} \\
        &= \begin{bmatrix}
            1 \\
            \M \phi_r(\M x)
        \end{bmatrix}^{\transpose}
        \begin{bmatrix}
            \M \phi^{\transpose}_r(\hat{\M x}){\bar{\M F}\bar{\M F}^{\transpose}}\M \phi_r(\hat{\M x}) & -\M \phi^{\transpose}_r(\hat{\M x}){\bar{\M F}\bar{\M F}^{\transpose}}\\
            -{\bar{\M F}\bar{\M F}^{\transpose}}\M \phi_r(\hat{\M x}) & {\bar{\M F}\bar{\M F}^{\transpose}}\\
        \end{bmatrix}
        \begin{bmatrix}
            1 \\
            \M \phi_r(\M x)
        \end{bmatrix} \\
        & = \|\M \phi_r(\M x) - \M \phi_r(\hat{\M x})\|^2_{{\bar{\M F}\bar{\M F}^{\transpose}}} \\
        % &= \|\M \phi_r(\M x) - \M \phi_r(\hat{\M x})\|^2_{\M{\Sigma}^{-1}}.
    \end{aligned}
    \end{equation}

    As $\bar{\M F}$ has full rank thus is bijective, $ \M s^{\transpose}\bar{\M F}\bar{\M F}^{\transpose}\M s = 0 \Leftrightarrow \bar{\M F}^{\transpose}\M s = 0 \Leftrightarrow \M s \in \operatorname{Null}(\bar{\M F}^{\transpose}) \Leftrightarrow \M s = 0 \Leftrightarrow {\bar{\M F}\bar{\M F}^{\transpose}}\succ 0$. Then we let $ \M{\Sigma} = ({\bar{\M F}\bar{\M F}^{\transpose}})^{-1}$ and we have the SOS belief: $$\|\M \phi_r(\M x) - \M \phi_r(\hat{\M x})\|^2_{\M{\Sigma}^{-1}}, \M{\Sigma} \succ 0.$$
    Furthermore, can see that the dual solution takes the form:
    \begin{equation}
        \hat{\M{Y}} = \begin{bmatrix}
            \M \phi^{\transpose}_r(\hat{\M x}){\bar{\M F}\bar{\M F}^{\transpose}}\M \phi_r(\hat{\M x}) & -\M \phi^{\transpose}_r(\hat{\M x}){\bar{\M F}\bar{\M F}^{\transpose}}\\
            -{\bar{\M F}\bar{\M F}^{\transpose}}\M \phi_r(\hat{\M x}) & {\bar{\M F}\bar{\M F}^{\transpose}}\\
        \end{bmatrix}.
    \end{equation}
\end{proof}

\section{Derivation of the Optimal Solution to BPUE under Constraints}
\label{appx:bpue-sos-cons}
\begin{theorem}[SOS Belief of Constrained BPUE]
For the constrained case that $\M x_k \in \mathcal{K}$, we have the modified SOS belief considering additional polynomial multipliers:
\begin{equation*}
    % \begin{aligned}
        \|\M \phi_r(\M x) - \M \phi_r(\hat{\M x})\|^2_{\M \Sigma^{-1}} = \|\M A \phi_r(\M x) - \M b\|^2_{\M V^{-1}} + \sum_j h_j(\M x)g_j(\M x).
\end{equation*}
with $\M{\Sigma}\succ 0$ and $h_j(\M{x})$ the multiplier. For feasible point $\M x_k \in \mathcal{K}$, we must have $g_j(\M x_k) = 0$, thus we have the equivalent covariance $\M{\Sigma}\succ 0$ on the support $\mathcal{K}$. 
 % \tsl{How about the constrained case? We need to restrict the system on the support $\mathbb{K}$. }
\end{theorem}
\begin{proof}
Under \Cref{assump:rank1sdp}, \Cref{theorem:SDP=POP}, we can construct the SOS belief by: % reformulate the objective function of \eqref{eq:BPUE} as an SOS belief: 
\begin{equation}
\begin{aligned}
    % L(\M x, \M \mu, \rho) 
    \M v^{\transpose}_r( \M x) \hat{\M Y} \M v_r(\M x) &=\|\M b - \M A\M \phi_r(\M x)\|^2_{\M{V}^{-1}} - \rho \\
    &  + \sum_i\mu_i\left\langle \M B_i^{\perp}, \M v_r( \M x)\M v^{\transpose}_r(\M x) \right \rangle \\
    & + \sum_{j} \lambda_{j} \left\langle \M G_{j}, \M v_r( \M x)\M v^{\transpose}_r(\M x)  \right\rangle,
\end{aligned}
\end{equation}
Consider the partition of the matrix $\M{B}^{\perp}$ and $\M{G}$:
\begin{equation}
    \M B^{\perp} =: \begin{bmatrix}
        0 & \M B^{\perp \intercal}_{l} \\
        \M B^{\perp}_{l}& \M B^{\perp}_{Q} 
    \end{bmatrix},    \M G =: \begin{bmatrix}
        0 & \M G^{\intercal}_{l} \\
        \M G_{l}& \M G_{Q} 
    \end{bmatrix}.
\end{equation}
% Using the multipliers obtained in the \eqref{prob:pop_sdp}, we have the \textit{dual solution} $\hat{\M Y}$:
The \textit{dual solution} $\hat{\M Y}$ takes the following form:
\begin{equation}
\label{eq:dual_sol_belief}
\hat{\M Y} = \begin{bmatrix} \M Y_c&\M Y_l^\transpose\\\M Y_l & \M Y_Q 
    \end{bmatrix}
\end{equation}
where
\begin{equation*}
\begin{aligned}
\M Y_c &= \M b^{\transpose}\M{V}^{-1}\M b - {\rho} \\
\M Y_l &= -{\M A}^{\intercal}\M{V}^{-1}{\M b} + \sum_i{\mu}_i \M B^{\perp}_{l, i}+ \sum_j{\lambda}_j \M G_{l, j}\\
\M Y_Q &= {\M A}^{\intercal}\M{V}^{-1}{\M A} + \sum_i {\mu}_i\M B_{Q,i}^{\perp} + \sum_j{\lambda}_j \M G_{Q, j}
\end{aligned}
\end{equation*}
By the structure of the SOS belief in \Cref{theorem:SDP=POP}, we have:
\begin{equation}
    \M{\Sigma}^{-1} = {\M A}^{\intercal}\M{V}^{-1}{\M A} + \sum_i {\mu}_i\M B_{ Q,i}^{\perp} + \sum_j{\lambda}_j \M G_{Q, j}.
\end{equation}
and we can further extract the optimal estimation by substituting $\M{b} = \M{A}\M{\phi}_r(\bar{\M{x}}) + \M{v}$:
\begin{equation}
\label{eq:BPUE_estimate_cons}
\begin{aligned}
   % &\M P\M \phi_r(\hat{\M x}) - {\M A}^{\intercal}\M{V}^{-1}{\M b} + \sum_i{\mu}_i \M B^{\perp}_{l, i} = 0 \\
    \quad\M \phi_r(\hat{\M x}) &= -\M{Y}_{Q}^{-1}\M{Y}_l \\
    % &\quad \color{gray} \text{\% $- \M{\Sigma}^{-1} \M \phi_r(\hat{\M x}) = \M Y_l $ by \Cref{theorem:SDP=POP}} \\
    &= {\M \Sigma} ({\M A}^{\intercal}\M{V}^{-1}{\M b} - \sum_i{\mu}_i \M B^{\perp}_{l, i} - \sum_j{\lambda}_j \M G_{l, j}) \\
    % &\quad \color{gray} \text{\% substituting $\M b = {\M A}\M \phi_r(\bar{\M x}) + \M v$ from \eqref{eq:gmm_cond}}\\
            &= {\M \Sigma}{\M A}^{\intercal}\M{V}^{-1}{\M A}\M \phi_r(\bar{\M x}) + {\M \Sigma}{\M A}^{\intercal}\M{V}^{-1}\M v \\
            & \quad - \sum_i{\mu}_i \M B^{\perp}_{l, i} -  \sum_j{\lambda}_j \M G_{l, j}
\end{aligned}
\end{equation}
Then we have the $$\delta\M{\phi} := \M{\Sigma}\M{A}^{\transpose}\M{V}^{-1}\M{v}$$
as we show in the unconstrained case. 
% For the derivation of the covariance approximation, in the constrained case that $\M x_k \in \mathcal{K}$, it is obvious to see that if we substitute $\M A = \bar{\M A}$ and $\M b = \bar{\M b} = \bar{\M A}\M \phi_r(\hat{\M x})$ to \eqref{eq:BPUE_dual_sol} and set $\M \mu = 0$ and $\M \lambda = 0$, the rest of the proof stays identical.

For the derivation of the approximated covariance under \Cref{assump:observability}, we follow the same steps in \Cref{sec:theory-covariance} to substitute $\M A = \bar{\M A}$ and $\M b = \bar{\M b} = \bar{\M A}\M \phi_r(\hat{\M x})$ in the noiseless case and set $\M \mu = 0$ and $\M \lambda = 0$. Then we have the identical result as the unconstrained case. 
\end{proof}

\section{Connection to Linear Kalman Filter}
\label{apx:linearkf}
\subsection{Recover the BLUE}
% \tsl{Low Priority: Derive the result given the certificate. }
We hereby compare the BPUE with BLUE and KF in the linear system without extended noise. Consider the linear dependency of $\M{v}$ term in \eqref{eq:BPUE_estimate}, we can generalize the gain of BLUE to the polynomial system considering the multipliers obtained from \eqref{prob:pop_sdp}:
\begin{definition}[Gain of BPUE]
    $$\M K_{uncon} = (\M A^{\transpose}\M{V}^{-1}\M A + \sum_i \mu_i \M B^{\perp}_{Q, i})^{-1}\M A^{\transpose}\M{V}^{-1}$$
    $$\M K_{cons} = (\M A^{\transpose}\M{V}^{-1}\M A + \sum_i \mu_i \M B^{\perp}_{Q, i} + \sum_i \lambda_i \M G^{\perp}_{Q, i})^{-1}\M A^{\transpose}\M{V}^{-1}.$$
\end{definition}

\subsection{Recover the Kalman gain}
Consider the optimization in the update steps with an SOS belief obtained from the previous step and an observation in the affine form:
\begin{equation}
    \min_{x \in \mathcal{K} }\quad \|\M \phi_r({\M x}) - \M \phi_r(\hat{\M x})\|^2_{\M{\Sigma}^{-1}} + \|\M b - \M A\M \phi_r(\M{x})\|^2_{\M{V}^{-1}}.
\end{equation}

Via the optimality condition \Cref{def:kkt_sdp} and \Cref{theorem:SDP=POP}, the dual solution with the same partition as \eqref{eq:dual_sol_belief} becomes:
\begin{equation*}
\begin{aligned}
\M Y_c &= \M{\phi}^{\transpose}_r(\hat{\M x})\M{\Sigma}^{-1}\M{\phi}_r(\hat{\M x}) + \M b^{\transpose}\M{V}^{-1}\M b - {\rho} \\
\M Y_l &=  -\M{\Sigma}^{-1}\M{\phi}_r(\hat{\M x}) -{\M A}^{\intercal}\M{V}^{-1}{\M b} + \sum_i{\mu}_i \M B^{\perp}_{l, i}+ \sum_j{\lambda}_j \M G_{l, j}\\
\M Y_Q &= \M{\Sigma}^{-1} + {\M A}^{\intercal}\M{V}^{-1}{\M A} + \sum_i {\mu}_i\M B_{Q,i}^{\perp} + \sum_j{\lambda}_j \M G_{Q, j}
\end{aligned}
\end{equation*}
By substituting $\M{b} = \M{A}\M{\phi}_r(\M{\bar{x}}) + \M{v}$ and extract the linear dependency of $\M{v}$, we can derive the generalized Kalman gain:
\begin{definition}[Generalized Kalman gain]
    $$\M K_{uncon} = (\M A^{\transpose}\M{V}^{-1}\M A + \M{\Sigma}^{-1} + \sum_i \mu_i \M B^{\perp}_{Q, i})^{-1}\M A^{\transpose}\M{V}^{-1}$$
    $$\M K_{cons} = (\M A^{\transpose}\M{V}^{-1}\M A + \M{\Sigma}^{-1} + \sum_i \mu_i \M B^{\perp}_{Q, i} + \sum_i \lambda_j \M G^{\perp}_{Q, j})^{-1}\M A^{\transpose}\M{V}^{-1}$$
\end{definition}
For unconstrained cases with $r=1$, all the multiplier vanishes and the gain reduces the classical Kalman gain.

\subsection{Covariance Update}
% We find that for unconstrained cases, the result reduces to BLUE with the classical Kalman gain. If we choose the operating point with noiseless measurement and prior, we have the equivalent propagation of covariance as:

Now we consider the update of covariance consider the dual solution $\M{Y}$. Let $\hat{\M\Sigma}^{+}_k = \M{Y}_Q$ and $\M\Sigma = \hat{\M\Sigma}_k^{-}$, we have the equivalent propagation of covariance considering the multiplier $\M{\mu}$ and $\M{\lambda}$ for the moment and localizing constraints: 
\begin{equation}
    (\hat{\M{\Sigma}}^{+}_{k})^{-1} = (\hat{\M{\Sigma}}^{-}_{k})^{-1} + \M A^{\transpose}\M V_k^{-1}\M A + \M{\xi} % \sum_i \mu_i\M B^{\perp}_{Q, i}
\end{equation}
For the unconstrained case:
\begin{equation}
    \M{\xi}_{uncon} = \sum_i \mu_i\M B^{\perp}_{Q, i}
\end{equation}
For the constrained case:
\begin{equation}
    \M{\xi}_{uncon} = \sum_i \mu_i\M B^{\perp}_{Q, i} + \sum_j \lambda_j\M G^{\perp}_{Q, j}
\end{equation}
% Via the matrix inversion lemma, we further have:
% \begin{equation}
%     \hat{\M{\Sigma}}^{+}_k = \hat{\M{\Sigma}}^{-}_k - \hat{\M{\Sigma}}^{-}_k((\M A^{\transpose}\M V_k^{-1}\M A + \M{\xi})^{-1} + \hat{\M{\Sigma}}^{-}_k)^{-1}\hat{\M{\Sigma}}^{-}_k.
%     \label{Cov_Update}
% \end{equation}

% \subsection{Propagation Steps}

\end{appendices}
\clearpage
