# Supplementary material for: GMKF: Generalized Moment Kalman Filter for Polynomial Systems with Arbitrary Noise
Source: arXiv:2403.04712 source file (2024-03-08)
Supplement: Supplementary file 2 [file Appendix.tex]

\clearpage

\begin{appendices}

\section{Examples of Auxiliary Matrices}
We now introduce two sets of matrix $\left\{\M{B}\right\}$ and $\left\{\M{B}^{\perp}\right\}$. We first introduce the auxiliary matrix $B_{\gamma}$ to form the moment matrix given the monomial $x^{\gamma}$:
\begin{equation}
    \M{B}_{\gamma} := \frac{1}{C_{\gamma}} \sum_{\gamma = \alpha + \beta} \ve_{\alpha} \ve^{\transpose}_{\beta},\ \  C_{\gamma}:= { \left| \left\{ (\alpha, \beta) | \gamma = \alpha + \beta \right\}  \right|  }
\end{equation}
where $\ve_\alpha \in \mathbb{R}^{s(r, n) \times 1}$ is the canonical basis corresponding to the $n$-tuples $\alpha \in \mathbb{N}_r^n$ and $C_{\gamma}$ is the normalizing factor. Thus, the moment matrix can be formulated by:
\begin{equation}
    \M{M}_r(\M x) = \sum_{\gamma} C_\gamma \M{B}_{\gamma} \M x^{\gamma}, \gamma \in \mathbb{N}^n_{2r}.
\end{equation}
% Conversely, we can extract the term of $\M{M}_r(y)$ via
% \begin{equation}
% x^{\gamma} = \langle B_\gamma, \M{M}_r(\M x) \rangle.
% \end{equation}
% We then define the orthogonal complement of $\left\{B\right\}$ considering the inner product as the trace function:
We define the symmetric matrix:
\begin{equation}
    \M{E}_{\alpha, \beta} = \ve_{\alpha}\ve_{\beta}^{\transpose} + \ve_{\beta}\ve_{\alpha}^{\transpose},
\end{equation}
and the orthogonal complement of $\left\{\M{B}\right\}$ to enforce the moment matrix constraints given an semidefinite matrix $X \ge 0$: 
\begin{equation}
   % \left\{ B^{\perp}_{\alpha, \beta} | \langle B^{\perp}_{\alpha, \beta}, B_{\alpha} \rangle, \forall \gamma \in \mathbb{N}^n_{2r} , \alpha + \beta = \gamma \right\}.
   \begin{aligned}
       &\M{B}^{\perp}_{\gamma, \alpha} = \M{E}_{\bar{\alpha}, \bar{\beta}} - \M{E}_{{\alpha}, {\beta}}, \\ 
       % &B^{\perp}_{\gamma, \alpha} = e_{\bar{\alpha}}e_{\bar{\beta}}^{\transpose} + e_{\bar{\beta}}e_{\bar{\alpha}}^{\transpose}  - e_{\alpha}e_{\beta}^{\transpose} - e_{\beta}e_{\alpha}^{\transpose}, \\ 
       &\alpha + \beta = \gamma, \alpha > \bar{\alpha}, \alpha \ge \beta, % \bar{\alpha} + \bar{\beta} = \gamma, 
   \end{aligned}
\end{equation}
where $\bar{\alpha} < \alpha$ is the tuple with the smallest possible lexical orders among all the $\alpha$. We provide a few examples of these matrices in \Cref{apx:B_mat_example}.
To assist the proof of our main theory, we introduce the following lemmas:

\section{Examples of moment matrix}
\label{apx:B_mat_example}
For $r = 2, n = 2$, we have the moment matrix:
\begin{equation}
    {\M M}_{2}(\M x) =\left[\begin{array}{cccccc}
1 & x_1 & x_2 & x_1^2 & x_1x_2 & x_2^2 \\
x_1 & x_1^2 & x_1x_2 & x_1^3 & x^2_1x_2 & x_1x_2^2 \\
x_2 & x_1x_2 & x^2_2 & x_1^2x_2 & x_1x^2_2 & x_2^3 \\
x_1^2 & x^3_1 & x_1^2x_2 & x_1^4 & x^3_1x_2 & x_1^2x_2^2 \\
x_1x_2 & x_1^2x_2 & x_1x^2_2 & x_1^3x_2 & x_1^2x_2^2 & x_1x_2^3 \\
x_2^2 & x_1x_2^2 & x^3_2 & x_1^2x_2^2 & x_1x^3_2 & x_2^4 \\
\end{array}\right] .
\end{equation} 
For $\gamma = (0, 2)$ that corresponds to $x_1^2$, we have:
\begin{equation}
    \M B_{\gamma} = \frac{1}{C_{\gamma}} \begin{bmatrix}
        0 & 0 & 0 & 1 & 0 & 0 \\
        0 & 1 & 0 & 0 & 0 & 0 \\
        0 & 0 & 0 & 0 & 0 & 0 \\
        1 & 0 & 0 & 0 & 0 & 0 \\
        0 & 0 & 0 & 0 & 0 & 0 \\
        0 & 0 & 0 & 0 & 0 & 0 \\
    \end{bmatrix}
\end{equation}
% \begin{equation}
%     B_{\gamma} = \frac{1}{C_{\gamma}} \begin{bmatrix}
%         0 & 0 & 0 & 0 & 1 & 0 \\
%         0 & 0 & 1 & 0 & 0 & 0 \\
%         0 & 1 & 0 & 0 & 0 & 0 \\
%         0 & 0 & 0 & 0 & 0 & 0 \\
%         1 & 0 & 0 & 0 & 0 & 0 \\
%         0 & 0 & 0 & 0 & 0 & 0 \\
%     \end{bmatrix}
% \end{equation}
and the $\left\{B^{\perp}\right\}$ as:
\begin{equation}
\begin{aligned}
    \M B^{\perp}_{\gamma, \alpha} &= \M e_{\bar{\alpha}}\M e_{\bar{\beta}}^{\transpose} + \M e_{\bar{\beta}}\M e_{\bar{\alpha}}^{\transpose}  - \M e_{\alpha}\M e_{\beta}^{\transpose} - \M e_{\beta}\M e_{\alpha}^{\transpose} \\
    &= \M E_{\bar{\alpha}, \bar{\beta}} - \M E_{{\alpha}, {\beta}} \\
    &= \begin{bmatrix}
        0 & 0 & 0 & -1 & 0 & 0 \\
        0 & 2 & 0 & 0 & 0 & 0 \\
        0 & 0 & 0 & 0 & 0 & 0 \\
        -1 & 0 & 0 & 0 & 0 & 0 \\
        0 & 0 & 0 & 0 & 0 & 0 \\
        0 & 0 & 0 & 0 & 0 & 0 \\
    \end{bmatrix}
\end{aligned}
\end{equation}
where have the following 
\begin{equation}
\begin{aligned}
     \M e_{\bar{\alpha}} &= \begin{bmatrix}
        0 & 1 & 0 & 0 & 0 & 0
    \end{bmatrix}, \M e_{\bar{\beta}} &= \begin{bmatrix}
        0 & 1 & 0 & 0 & 0 & 0
    \end{bmatrix},\\
    \M e_{{\alpha}} &= \begin{bmatrix}
        0 & 0 & 0 & 1 & 0 & 0
    \end{bmatrix}, \M e_{{\beta}} &= \begin{bmatrix}
        1 & 0 & 0 & 0 & 0 & 0
    \end{bmatrix}. \\
\end{aligned}
\end{equation}
Via enforcing the constraints:
\begin{equation}
    \langle \M B^{\perp}_{\gamma, \alpha}, \M X \rangle = 0, \M X \ge 0
\end{equation}
we can guarantee that all the entries corresponding to $x_1^2$ are identical. 
% \begin{equation}
% \begin{aligned}
%     B_{\gamma, \alpha_1} &= \begin{bmatrix}
%         0 & 0 & 0 & -1 & 0 & 0 \\
%         0 & 1 & 0 & 0 & 0 & 0 \\
%         0 & 0 & 0 & 0 & 0 & 0 \\
%         0 & 0 & 0 & 0 & 0 & 0 \\
%         0 & 0 & 0 & 0 & 0 & 0 \\
%         0 & 0 & 0 & 0 & 0 & 0 \\
%     \end{bmatrix} \\ 
%     B_{\gamma, \alpha_2} &= \begin{bmatrix}
%         0 & 0 & 0 & 0 & 0 & 0 \\
%         0 & 1 & 0 & 0 & 0 & 0 \\
%         0 & 0 & 0 & 0 & 0 & 0 \\
%         -1 & 0 & 0 & 0 & 0 & 0 \\
%         0 & 0 & 0 & 0 & 0 & 0 \\
%         0 & 0 & 0 & 0 & 0 & 0 \\
%     \end{bmatrix}
% \end{aligned}
% \end{equation}

\section{Proof of Lemma \ref{lemma:B_orthogonal}}
\label{apx:proof:B_orthogonal}
% \begin{lemma}
%     All $B^{\perp}$ and $B$ forms a basis for matrix $\mathbb{R}^{s(r, n) \times s(r, n)}$ and they are orthogonal complement.
% \end{lemma}
\begin{proof}
To show the orthogonality, we have:
\begin{equation}
\label{eq:B_orthogonal}
\begin{aligned}
    \left\langle \M B_{\gamma, \alpha}^{\perp}, \M B_{\gamma} \right\rangle &= \langle \M E_{\bar{\alpha}, \bar{\beta}} - \M E_{{\alpha}, {\beta}},  \frac{1}{C_{\gamma}} \sum_{\gamma = \alpha' + \beta'} \M e_{\alpha'} \M e^{\transpose}_{\beta'} \rangle \\
    &= \langle \M e_{\bar{\alpha}}\M e_{\bar{\beta}}^{\transpose} + \M e_{\bar{\beta}}\M e_{\bar{\alpha}}^{\transpose},  \frac{1}{C_{\gamma}} \sum_{\gamma = \alpha' + \beta'} \M e_{\alpha'} \M e^{\transpose}_{\beta'}\rangle \\ & \quad -  \langle \M e_{{\alpha}}\M e_{{\beta}}^{\transpose} + \M e_{{\beta}}\M e_{{\alpha}}^{\transpose},  \frac{1}{C_{\gamma}} \sum_{\gamma = \alpha' + \beta'} \M e_{\alpha'} \M e^{\transpose}_{\beta'} \rangle \\
    & = \frac{2}{C_{\gamma}} - \frac{2}{C_{\gamma}} = 0
\end{aligned}
% \begin{aligned}
%     \left\langle B^{\perp}_{\gamma, \alpha}, M_r(x) \right\rangle &= \langle B^{\perp}_{\gamma, \alpha}, \sum_{\gamma} C_\gamma B_{\gamma} x^{\gamma}\rangle = 0  \\
%       & \Rightarrow \left\langle B^{\perp}_{\gamma, \alpha}, B_{\gamma} \right\rangle = 0 \\
% \end{aligned}
\end{equation} % , \gamma
% \tsl{Add a remark that $B$ and $B^{\perp}$ are sufficient to generate any matrix.} \tsl{$B$ and $B^{\perp}$ are orthogonal to each other and can generate any matrix, thus is an element-wise basis.}
To show $\left\{\M B\right\} \cup \left\{\M B^{\perp}\right\}$ form a basis for symmetric matrix $\mathbb{R}^{s(r, n) \times s(r, n)}$, given the $\bar{\alpha}$ and $\bar{\beta}$, we have:
\begin{equation}
\label{eq:B_basis}
    \M e_{\bar{\alpha}}\M e^{\transpose}_{\bar{\beta}} = C_{\gamma}\M B_{\gamma} - \sum_{\gamma = \alpha + \beta}\M e_{\alpha}\M e_{\beta}^{\transpose}
\end{equation}
\begin{equation}
\label{eq:E_alpha_beta}
\begin{aligned}
    \M E_{\bar{\alpha}, \bar{\beta}} &= 2C_{\gamma}\M B_{\gamma} - \sum_{\gamma = \alpha + \beta, \alpha \ge \beta}\M E_{\alpha, \beta} \\
    &= 2C_{\gamma}\M B_{\gamma} - \sum_{\gamma = \alpha + \beta, \alpha \ge \beta}(\M B^{\perp}_{\gamma, \alpha} - \M E_{\bar{\alpha}, \bar{\beta}})
\end{aligned}
\end{equation}
% \begin{equation}
% \begin{aligned}
%     E_{\bar{\alpha}, \bar{\beta}} = 2C_{\gamma}B_{\gamma} - \sum_{\gamma = \alpha + \beta, \alpha \ge \beta}(B^{\perp}_{\gamma, \alpha} - E_{\alpha, \beta})
% \end{aligned}
% \end{equation}

% \begin{equation}
% \label{eq:B_basis}
% \begin{aligned}
%     e_{\bar{\alpha}}e^{\transpose}_{\bar{\beta}} &= C_{\gamma}B_{\gamma} - \sum_{\gamma = \alpha + \beta}e_{\alpha}e_{\beta}^{\transpose} \\
%     &= C_{\gamma}B_{\gamma} + \sum_{\gamma = \alpha + \beta}(B^{\perp}_{\gamma, \alpha} - e_{\bar{\alpha}}e^{\transpose}_{\bar{\beta}}) \\
%     (C_{\gamma} + 1)e_{\bar{\alpha}}e^{\transpose}_{\bar{\beta}} &= C_{\gamma}B_{\gamma} + \sum_{\gamma = \alpha + \beta}B^{\perp}_{\gamma, \alpha} \\
%     % e_{\bar{\alpha}}e^{\transpose}_{\bar{\beta}} &= \frac{C_{\gamma}}{(C_{\gamma} + 1)} B_{\gamma} + \frac{1}{(C_{\gamma} + 1)}\sum_{\gamma = \alpha + \beta}B^{\perp}_{\gamma, \alpha}
% \end{aligned}
% \end{equation}

Thus, $\forall \alpha, \beta$ and $\alpha + \beta = \gamma$, we have:
\begin{equation}
\begin{aligned}
    \M E_{\alpha, \beta} &= \M E_{\bar{\alpha}, \bar{\beta}} - \M B^{\perp}_{\gamma, \alpha}
    % &=\frac{C_{\gamma}}{(C_{\gamma} + 1)} B_{\gamma} + \frac{1}{(C_{\gamma} + 1)}\sum_{\gamma = \alpha' + \beta'}B^{\perp}_{\gamma, \alpha'} - B_{\gamma, \alpha}^{\perp}
\end{aligned}
\end{equation}
By substituting \eqref{eq:E_alpha_beta}, we show that any entry of the symmetric matrix can be represented by the linear combination of elements in $\left\{\M B\right\} \cup \left\{\M B^{\perp}\right\}$. \tsl{Need to check the constant.}
\end{proof}

\section{Proof of Lemma \ref{lemma:exist_sos_xi}}
\label{apx:proof:exist_sos_xi}
% Before the main theorem, we introduce the lemma about the equivalence of the dual certificate:
% \begin{lemma}[Equivalent polynomial]
%     \label{lemma:exist_sos_xi}
%     Let $Y_1$ and $Y_2$ be two matrices such that $v^{\transpose}_r(\M x) Y_1 v^{\transpose}_r(\M x)=v^{\transpose}_r(\M x) Y_2 v^{\transpose}_r(\M x)$ for all $x$, i.e., the polynomials corresponding to $Y_1$ and $Y_2$ are identical. Then there exists a matrix ${\xi}$ with $\left\langle{\xi}, {B}_{{\gamma}}\right\rangle=0$ for all ${\gamma}$ such that $Y_1=Y_2+{\xi}$. % and $\xi = \sum_{(\gamma, \alpha)}\mu_{\gamma, \alpha}B_{\gamma, \alpha}^{\perp}$.
% \end{lemma}
% \begin{lemma}[Equivalent polynomial]
%     \label{lemma:exist_sos_xi}
%     Let $\M{Y}_1$ and $\M{Y}_2$ be two matrices such that $\vv^{\transpose}_r(\M x) \M{Y}_1 \vv^{\transpose}_r(\M x)=\vv^{\transpose}_r(\M x) \M{Y}_2 \vv^{\transpose}_r(\M x)$ for all $x$, i.e., the polynomials corresponding to $\M{Y}_1$ and $\M{Y}_2$ are identical. Then there exists a matrix ${\xi}$ with $\left\langle{\M{\xi}}, {\M{B}}_{{\gamma}}\right\rangle=0$ for all ${\gamma}$ such that $\M{Y}_1=\M{Y}_2+{\M{\xi}}$, $\M{\xi}=\sum_{(\gamma, \alpha)} \mu_{\gamma, \alpha} \M{B}^{\perp}_{\gamma, \alpha}$. % and $\xi = \sum_{(\gamma, \alpha)}\mu_{\gamma, \alpha}B_{\gamma, \alpha}^{\perp}$.
% \end{lemma}
\begin{proof}
        \begin{align}
        &\M v^{\transpose}_r(\M x) (\M Y_1-\M Y_2) \M v_r( \M x)=0, \quad \forall \M x \Leftrightarrow  \\
        &\left\langle \M Y_1-\M Y_2, \M v_r( \M x)\M v^{\transpose}_r(\M x)\right\rangle=0, \quad \forall \M x \Leftrightarrow \\
        &\langle \M Y_1-\M Y_2, \sum \M x^{\gamma}\M B_{\gamma}\rangle=0, \quad \forall \M x \Rightarrow \\
        &\left\langle \M Y_1-\M Y_2, {\M B}_{{\gamma}}\right\rangle= 0, \quad \forall \gamma
        \end{align}
% This last implication holds in the reverse direction: if a polynomial $p(\mathbf{z})$ has all zero coefficients, then it must be the zero polynomial.
As $\left\{\M B^{\perp}\right\}$ and $\left\{\M B\right\}$ are orthogonal complements, $\xi$ exist and can be constructed by $\M B^{\perp}$ as
    \begin{equation}
    \label{eq:exist_of_xi}
        \M Y_1 - \M Y_2 = \sum_{(\gamma, \alpha)} \mu_{\gamma, \alpha} \M B^{\perp}_{\gamma, \alpha} =: \M \xi .
    \end{equation}
\end{proof}

\section{Proof of \Cref{lemma:dual_matrix}}
\begin{equation}
    \begin{aligned}
        &\langle \M Y, \M X \rangle = \langle \M Y, \M v_r(\M x)\M v^{\transpose}_r(\M x) \rangle = \M v^{\transpose}_r(\M x)\M Y\M v_r(\M x) \\
    \end{aligned}
    \end{equation}
    We also have
    \begin{equation}
    \begin{aligned}
        \langle \M Y, \M X \rangle
        &=  \left\langle \M C + \sum_{i} \lambda_{i} \M G_{i} + \left( \sum_{j}\mu_{j} \M B^{\perp}_{j} - \rho \M e_1\M e_1^{\transpose} \right), \M X \right\rangle \\
        &= \langle \M C,  \M X \rangle + 
        \langle \sum_{i} \lambda_{i} \M G_{i} , \M X \rangle + \\
        & \langle\sum_{j}\mu_{j} \M B^{\perp}_{j} , \M X \rangle - \langle \rho \M e_1\M e_1^{\transpose}, \M X \rangle \\
        &= \langle \M C,  \M X \rangle + 
        \langle\sum_{j}\mu_{j} \M B^{\perp}_{j} , \M X \rangle - \langle \rho \M e_1\M e_1^{\transpose}, \M X \rangle \\
        &= \langle \M C,  \M X \rangle + 
        \sum_{j}\mu_{j} \langle \M B^{\perp}_{j} , \M v_r(\M x)\M v^{\transpose}_r(\M x) \rangle - \rho \\
        % &= p(\M x) - \rho + \sum_{i=1}^{m} g_i(\M x)h_i(\M x) .
        % &= \langle \M P + \sum_{i}\lambda_{i} \M G_{i}, \M X \rangle -\rho \langle \M e_1\M e_1^{\transpose}, \M X\rangle + \sum_{j}\mu_{j} \langle \M B_{j}^{\perp}, \M X \rangle \\
        % &= \langle \M C + \sum_{i}\lambda_{i} \M G_{i}, \M X \rangle - \rho ,
    \end{aligned}
    \end{equation}

\section{Proof of Theorem \ref{theorem:SDP=POP}}
\label{apx:SDP=SOS}

% 0Now we show that, under the rank-1 assumption, the SoS form induced from the optimality condition can be used to construct the prior factor in the moment matching problem. 

Now, it suffices to show the equivalence of the SDP primal solution and the duality certificate.
% \tsl{Need to show why it is sufficient to construct $\xi$ by $B^{\perp}$ .} \tsl{Need some basis theorem maybe.}
% \begin{theorem}[Dual certificate as the prior factor]
%     % The \ref{SDP} has rank-1 optimal solutions if and only if the SOS global optimality condition is satisfied and $\sigma_0(x)$ is an prior factor of the moment matching problem.
%     % Suppose that the solution
%     % The dual SOS $\sigma_0(x)$ is in the form of prior factor if and only if the first-order optimality condition is satisfied. 
%     Suppose the unique optimal solution of \ref{prob:pop} is $\bar{x}$. The \ref{prob:pop_sdp} corresponding to \ref{prob:pop} has rank-1 optimal solution $v_r(\bar{x})v_r(\bar{x})^{\transpose}$. Then the dual certificate is of the form \mbox{$\sigma_0(x) = \| v_r(\M x) - v_r(\bar{x}) \|_{W}^2$}, $W>0$, iff the first order optimality condition \ref{def:kkt_sdp} is satisfied. 
% \end{theorem}
\begin{proof}
    The only if part. 
    Suppose $\sigma_0$ has the form:
    \begin{equation}
        \begin{aligned}
        \sigma_0(\M x) &= \|\M \phi_r(\M x) - \M \phi_r(\bar{\M x})\|^2_{\M W} \\
                    &= p(\M x) + \sum_{k=1}^m h_i(\M x)g_i(\M x) - \rho, \M W > 0 
        \end{aligned}
    \end{equation}
    We have: % Can be expanded as a $s(r, n)\times s(r, n)$ to serve as the dual certificate. 
    \begin{equation}
        \begin{aligned}
            & \sigma_0(\M x) = \M v^{\transpose}_r(\M x)\M Y\M v_r(\M x) \\
            &=\begin{bmatrix}
            1 \\
            \M \phi_r(\M x)
        \end{bmatrix}^{\transpose}
        \begin{bmatrix}
             \M \phi_r(\bar{\M x})^{\transpose}W\M \phi_r(\bar{\M x}) & -(\M W\M \phi_r(\bar{\M x}))^{\transpose} \\
            -\M W\M \phi_r(\bar{\M x}) & \M W
        \end{bmatrix}\begin{bmatrix}
            1 \\
            \M \phi_r(\M x)
        \end{bmatrix}
        \end{aligned}
    \end{equation}
    The dual certificate can be constructed as 
    $$\M Y:= \begin{bmatrix}
        \M \phi_r(\bar{\M x})^{\transpose}\M W\M \phi_r(\bar{\M x}) & -(\M W\M \phi_r(\bar{\M x}))^{\transpose} \\
            -\M W\M \phi_r(\bar{\M x}) & \M W
        \end{bmatrix}$$
    and primal solution is:
    $$
        \M X:= \begin{bmatrix}
            1 \\
            \M \phi_r(\bar{\M x})
        \end{bmatrix}\begin{bmatrix}
            1 \\
            \M \phi_r(\bar{\M x})
        \end{bmatrix}^{\transpose}.
    $$
    It is straightforward to verify that $Rank(\M X) = 1$, $Rank(\M Y) = s(r, n) - 1$, and $\langle \M X, \M Y \rangle = 0$. 
    Given the construction of the SoS, we have
    $$\M v^{\transpose}_r(\M x)\M Y\M v_r(\M x) = \M v^{\transpose}_r\left(\M P -\rho \M e_1\M e_1^{\transpose} + \sum_{(i, \beta)} \lambda_{i, \beta} \M G_{i, \beta}\right)\M v_r(\M x).$$ By Lemma \ref{lemma:exist_sos_xi}, there must exist $\xi = \sum_{(\gamma, \alpha)} \mu_{\gamma, \alpha} \M B^{\perp}_{\gamma, \alpha}$ that enable the construction of the first-order optimality condition: 
    $$\M Y = \M P - \rho \M e_1\M e_1^{\transpose} + \sum_{(i, \beta)} \lambda_{i, \beta} \M G_{i, \beta} + \M \xi.$$
    % \tsl{$\rho$ is missed here.}
    
    The if part.
    If the SDP has a rank-1 solution and satisfies the strict complementary condition, we have $\langle X, Y\rangle = 0$, with $Rank(X) = 1, Rank(Y) = s(r, n) - 1$. By SVD of $Y$, we have:
    % $$Y = \sum_{i=1}^{s(r, n) - 1} \delta_i f_if_i^{\transpose}, \delta_i > 0, $$
    \begin{equation}
        \begin{aligned}
            \M Y &= \sum_{i=1}^{s(r, n) - 1} \delta_i \M f_i\M f_i^{\transpose} \\
              &= \begin{bmatrix}
                  \sqrt{\delta_1}\M f^{\transpose}_i \\
                  \vdots \\
                  \sqrt{\delta_{s(r, n) - 1}}\M f^{\transpose}_{{s(r, n) - 1}} \\
              \end{bmatrix}^{\transpose}
              \begin{bmatrix}
                  \sqrt{\delta_1}\M f^{\transpose}_i \\
                  \vdots \\
                  \sqrt{\delta_{s(r, n) - 1}}\M f^{\transpose}_{{s(r, n) - 1}} \\
              \end{bmatrix} \\
              &=: \M F\M F^{\transpose},
        \end{aligned}
    \end{equation}
    with $\M F \in \mathbb{R}^{s(r, n)\times\left( s(r, n) - 1 \right)}$ and $\delta_i > 0$ the non-trivial singular values. Similarly, by SVD of $\M X$ and $\langle \M X, \M Y \rangle = 0$, we have:
    \begin{equation}
        \M X =  \begin{bmatrix}
            1 \\
            \M \phi_r(\bar{\M x})
        \end{bmatrix}\begin{bmatrix}
            1 \\
            \M \phi_r(\bar{\M x})
        \end{bmatrix}^{\transpose}, \begin{bmatrix}
            1 \\
            \M \phi_r(\bar{\M x})
        \end{bmatrix}^{\transpose}\M f_i = 0 .
    \end{equation}
Let us extract the first row of $\M F$ as $\M f$ and define:
    \begin{equation}
        \M F = \begin{bmatrix}
            \M f \\
            \bar{\M F}
        \end{bmatrix}, \M f\in\mathbb{R}^{1\times (s(r,n) - 1) }, \bar{\M F} \in \mathbb{R}^{(s(r, n) - 1) \times (s(r, n) - 1) }
    \end{equation}
     By the strict complementary condition, we have
    \begin{equation}
        \M F^{\transpose}\begin{bmatrix}
            1 \\
            \M \phi_r(\bar{\M x})
        \end{bmatrix} = \begin{bmatrix}
            \M f^{\transpose}, \bar{\M F}^{\transpose}
        \end{bmatrix}\begin{bmatrix}
            1 \\
            \M \phi_r(\bar{\M x})
        \end{bmatrix} = \M f^{\transpose} + \bar{\M F}^{\transpose}
            \M \phi_r(\bar{\M x}) = 0
    \end{equation}
    \begin{equation}
        \M f^{\transpose} = - \bar{\M F}^{\transpose}\M \phi_r(\bar{\M x})
    \end{equation}
    As ${\M f}^{\transpose}$ is a linear combination of the $\bar{\M F}$, $\bar{\M F}$ must have full rank to ensure that $Rank(\M F) = s(r, n) - 1$.

    % Thus, the dual certificate $Y$ can construct the prior factor
    Then we obtain the SOS of $Y$ via:
    \begin{equation}
    \begin{aligned}
        \sigma_0(\M x) &= \begin{bmatrix}
            1 \\
            \M \phi_r(\M x)
        \end{bmatrix}^{\transpose}\M Y\begin{bmatrix}
            1 \\
            \M \phi_r(\M x)
        \end{bmatrix} \\
        & = \begin{bmatrix}
            1 \\
            \M \phi_r(\M x)
        \end{bmatrix}^{\transpose}\M F\M F^{\transpose}\begin{bmatrix}
            1 \\
            \M \phi_r(\M x)
        \end{bmatrix} \\
        &= \begin{bmatrix}
            1 \\
            \M \phi_r(\M x)
        \end{bmatrix}^{\transpose}
        \begin{bmatrix}
            \M f\M f^{\transpose} & \M f\bar{\M F}^{\transpose} \\
            \bar{\M F}\M f^{\transpose} & \bar{\M F} \bar{\M F}^{\transpose}\\
        \end{bmatrix}
        \begin{bmatrix}
            1 \\
            \M \phi_r(\M x)
        \end{bmatrix} \\
        &= \begin{bmatrix}
            1 \\
            \M \phi_r(\M x)
        \end{bmatrix}^{\transpose}
        \begin{bmatrix}
            \M \phi^{\transpose}_r(\bar{\M x})\bar{\M F}\bar{\M F}^{\transpose}\M \phi_r(\bar{\M x}) & -\M \phi^{\transpose}_r(\bar{\M x})\bar{\M F}^{\transpose}\bar{\M F}\\
            -\bar{\M F}\bar{\M F}^{\transpose}\M \phi_r(\bar{\M x}) & \bar{\M F} \bar{\M F}^{\transpose}\\
        \end{bmatrix}
        \begin{bmatrix}
            1 \\
            \M \phi_r(\M x)
        \end{bmatrix} \\
        & = \|\M \phi_r(\M x) - \M \phi_r(\bar{\M x})\|^2_{\bar{\M F}\bar{\M F}^{\transpose}}
    \end{aligned}
    \end{equation}

    As $\bar{\M F}$ has full rank thus bijective, $ \M s^{\transpose}\bar{\M F}\bar{\M F}^{\transpose}\M s = 0 \Leftrightarrow \bar{\M F}^{\transpose}\M s = 0 \Leftrightarrow \M s \in \operatorname{Null}(\bar{\M F}^{\transpose}) \Leftrightarrow \M s = 0 \Leftrightarrow {\bar{\M F}\bar{\M F}^{\transpose}} > 0$.
\end{proof}

\section{Connection to linear KF}
%%%%%%%%%%%%%%%%%%%%%% Connection to KF %%%%%%%%%%%%%%%%%%%%%%
Then we can define the generalized BLUE with multipliers induced from the moment relaxation:
\begin{definition}[Gain of BPUE]
    $$\M K = (\M A^{\transpose}\M W\M A + \sum_i \mu_i \M B^{\perp}_{Q, i})^{-1}\M A^{\transpose}\M W$$
\end{definition}
Consider the Lagrangian of the SDP in the update steps with noiseless SOS factor:
\begin{equation}
\label{eq:KF_local_kkt}
\begin{aligned}
    L(\M m, \M \mu) = & \|\M \phi_r({x}) - \M \phi_r(\bar{x})\|^2_{\M P} + \|\M b - \M A\M \phi_r({x})\|^2_\M W \\
    &+ \sum_i\mu_i\langle \M B_i^{\perp}, \M m_e\M m_e^{\intercal}\rangle  % // + \rho\left(\langle e_1e^\intercal_1, m_em_e^{\intercal}\rangle - 1\right)  \\
\end{aligned}
\end{equation}
we can derive the generalized Kalman gain:
\begin{definition}[Generalized Kalman gain]
    $$\M K = (\M A^{\transpose}\M W\M A + \M P + \sum_i \mu_i \M B^{\perp}_{Q, i})^{-1}\M A^{\transpose}\M W$$
\end{definition}
\LC{also this is very unclear: we derive the gain K but that's not actually used by that algorithm?}
For the unconstrained linear optimal estimator, the multipliers vanish and degenerate to the BLUE and linear KF. 

We find that for unconstrained cases, the result reduces to BLUE with the classical Kalman gain. \tsl{This is not Kalman gain... Kalman gain has a P matrix inside the ()}
If we consider the cost function as in the update steps, we have the estimation as:
\begin{equation}
\begin{aligned}
    \hat{\M m} &= ({A}^{\intercal}W{A} + P + \sum_i {\mu}_iB_{Q,i}^{\perp})^{-1}({A}^{\intercal}W{b} + Pm^{-} - \sum_i{\mu}_i B^{\perp}_{l, i}) \\
            &=\bar{\M m} + ({A}^{\intercal}W{A} + P + \sum_i {\mu}_iB_{Q,i}^{\perp})^{-1}({A}^{\intercal}W(A\bar{\M m} + v) + Pm^{-} - \sum_i{\mu}_i B^{\perp}_{l, i}) \\
\end{aligned}
\end{equation}
\label{appx:mkf_cov_update}
We find that for unconstrained cases, the result reduces to BLUE with the classical Kalman gain. If we choose the operating point with noiseless measurement and prior, we have the equivalent propagation of covariance as:
\begin{equation}
    (\hat{\M P}^{+}_{k})^{-1} = (\hat{\M P}^{-}_{k})^{-1} + \M A^{\transpose}\M V_k^{-1}\M A  
\end{equation}
via the matrix inversion lemma, we can recover the classical result in Kalman filter:
\begin{equation}
    \hat{\M P}^{+}_k = \hat{\M P}^{-}_k - \hat{\M P}^{-}_k\M A^{\transpose}(\M V_k + A\hat{\M P}^{-}_k\M A^{\transpose})^{-1}\M A\hat{\M P}^{-}_k
\end{equation}
In the noisy case and assuming the rank one solution is available, we have the equivalent propagation of covariance considering the multiplier $\mu_i$ and the matrix $\M B^{\perp}$:
\begin{equation}
    (\hat{\M P}^{+}_{k})^{-1} = (\hat{\M P}^{-}_{k})^{-1} + \M A^{\transpose}\M V_k^{-1}\M A + \sum_i \mu_i\M B^{\perp}_{Q, i}
\end{equation}
\begin{equation}
    \hat{\M P}^{+}_k = \hat{\M P}^{-}_k - \hat{\M P}^{-}_k\left((\M A^{\transpose}\M V_k^{-1}\M A + \sum_i \mu_i\M B^{\perp}_{Q, i})^{-1} + \hat{\M P}^{-}_k\right)^{-1}\hat{\M P}^{-}_k
    \label{Cov_Update}
\end{equation}
We will show in the next section that the multipliers $\mu_i$ result in equivalent polynomials.

\end{appendices}
